# Supplementary material for: Resonance fluorescence in a waveguide geometry
Source: arXiv:1111.7315 ancillary file (2012-02-16)
Supplement: Supplementary file 1 [file resFl_final.pdf]

# Mathematica Notebook for Analytically Calculating Various Expectation Values

---

## Preamble

```
In[1]:= (* Clears previous declarations, and sets up the environment. *)
x = x; Remove["Global`*"];
Off[General::spell];
Off[General::spell1];
<< "AuthorTools`"
SetDirectory[NotebookFolder[EvaluationNotebook[]]];
```

---

## Derivation of analytical formulas

### ■ Definitions

The code below is based on

The Mathematica Guidebook for Programming (Springer, 2004) by Michael Trott

Sec. 5, Exercise 8 : Operator Product

<http://www.mathematicaguidebooks.org/toc.shtml>

```
In[6]:= (* If the symbol has an OverBar, i.e.  $\overline{x}$ , it is an operator *)
notOperatorQ[φ_] := FreeQ[φ, _OverBar];
operatorQ[φ_] := !notOperatorQ[φ];
(* Associativity (OP stands for operator product) *)
OP[a___, OP[b___], c___] := OP[a, b, c]
(* Additivity *)
OP[a___, b1_ + b2_, c___] := OP[a, b1, c] + OP[a, b2, c]
(* overBar independent expressions are not operators *)
OP[x_?notOperatorQ] := x
(* factor out OverBar independent factors *)
OP[a___, x_?notOperatorQ, b___] := x OP[a, b]
OP[a___, x_?notOperatorQ y_, b___] := x OP[a, y, b]
(* multiply out powers of sums *)
OP[a___, b_Plus^n_Integer?(> 1 &), c___] :=
  OP[a, Table[b, {n}] /. List -> Sequence, c]
(* to reduce the notation,
```

```

write products of operators as powers (this may not always be desirable) *)
OP[a___, OverBar[x_]^n1_., OverBar[x_]^n2_., c___] :=
OP[a, OverBar[x]^ (n1 + n2), c]
(* single operators are not operator products *)
OP[OverBar[a_]] := OverBar[a];

(* Now, let us define the averaging
operator <x> using the AngleBracket[] symbol *)
(* Averaging works on single items, not on lists *)
(* Associativity *)
AngleBracket[AngleBracket[b_]] := AngleBracket[b]
(* Additivity *)
AngleBracket[b1_ + b2_] := AngleBracket[b1] + AngleBracket[b2]
(* overBar independent expressions are
not operators and are equal to their averages *)
AngleBracket[x_?notOperatorQ] := x
(* factor out OverBar independent factors *)
AngleBracket[x___?notOperatorQ y_] := x AngleBracket[y]

(* These are the specific rules for simplification *)
(* Take out input operators at the outer periphery *)
AngleBracket[OverBar[ad[t_]]] :=  $\frac{\omega 0}{2} \sqrt{\frac{\tau'}{2}} e^{-i\phi} e^{ikt}$ ;
AngleBracket[HoldPattern[OP[OverBar[ad[t_]], c___]]] :=
 $\frac{\omega 0}{2} \sqrt{\frac{\tau'}{2}} e^{-i\phi} e^{ikt}$  AngleBracket[OP[c]];
AngleBracket[OverBar[a[t_]]] :=  $\frac{\omega 0}{2} \sqrt{\frac{\tau'}{2}} e^{+i\phi} e^{-ikt}$ ;
AngleBracket[HoldPattern[OP[c___, OverBar[a[t_]]]]] :=
 $\frac{\omega 0}{2} \sqrt{\frac{\tau'}{2}} e^{+i\phi} e^{-ikt}$  AngleBracket[OP[c]];

(* Commutator relations between a, ad=a†, sm=σ-, sp=σp *)
OP[c___, OverBar[a[t1_]], OverBar[sm[t2_]], d___] :=
OP[c, OverBar[sm[t2_]], OverBar[a[t1_]], d] /;
Refine[t1 >= t2, Element[t1, Reals] && Element[t2, Reals]]
OP[c___, OverBar[sp[t2_]], OverBar[ad[t1_]], d___] :=
OP[c, OverBar[ad[t1_]], OverBar[sp[t2_]], d] /;
Refine[t1 >= t2, Element[t1, Reals] && Element[t2, Reals]]

(* sp[t] sm[t] = (sz[t]+1)/2 *)
OP[c___, OverBar[sp[t_]], OverBar[sm[t_]], d___] :=  $\frac{1}{2}$  OP[c, OverBar[sz[t]] + 1, d]

(* Code bleow is not necessary unless numerical solutions are required---
see previous notebook versions *)

```

```

(*)
(* Two time averages should have the larger time to the right *)
AngleBracket[HoldPattern[OP[OverBar[sp[t1_]],OverBar[sm[t2_]]]]:=
Conjugate[AngleBracket[OP[OverBar[sp[t2_]],OverBar[sm[t1_]]]]/;
  Refine[t1>t2,Element[t1,Reals]&& Element[t2,Reals]]
  AngleBracket[HoldPattern[OP[OverBar[sm[t1_]],OverBar[sm[t2_]]]]:=
Conjugate[AngleBracket[OP[OverBar[sp[t2_]],OverBar[sp[t1_]]]]/;
  Refine[t1>t2,Element[t1,Reals]&& Element[t2,Reals]]
  AngleBracket[HoldPattern[OP[OverBar[sz[t1_]],OverBar[sm[t2_]]]]:=
Conjugate[AngleBracket[OP[OverBar[sp[t2_]],OverBar[sz[t1_]]]]/;
  Refine[t1>t2,Element[t1,Reals]&& Element[t2,Reals]]
*)

(* Some tests of the symbolic parts *)
(* Various tests for the operators, and the expectation values.
For debugging purposes, Trace[] and Stack[] commands are useful.
Change the False below to True to evaluate the expressions. *)
If[False,
  OP[1 +  $\bar{t}$  +  $\bar{z}^2$ ]
  OP[2,  $\bar{t}$ ,  $\bar{z}^2$ , r,  $\bar{u}$ ]
  OP[( $\bar{s} + \bar{k}$ )^2]
   $\langle 1 + \bar{t} + \bar{z}^2 \rangle$ 
   $\langle x + 3 y \bar{t} \rangle$ 
   $\langle OP[(\bar{s} + \bar{k})^2] \rangle$ 
   $\langle OP[\overline{ad[t]}, \bar{x}, \bar{y}] \rangle$ 
   $\langle OP[\bar{x}, \bar{y}, \overline{ad[t]}] \rangle$ 
   $\langle OP[\bar{x}, \bar{y}, \overline{a[t]}] \rangle$ 
   $\langle OP[\overline{a[t]}, \overline{sm[t]}] \rangle$ 
   $\langle OP[\overline{ad[t]}, \overline{sm[t]}] \rangle$ 
   $\langle OP[\overline{sp[t]}, \overline{ad[t-1]}] \rangle$ 
   $\langle OP[\overline{ad[t]}] \rangle$ 
   $\langle OP[\overline{a[t]}] \rangle$ 
  Assuming[x > 0,  $\langle OP[\overline{a[t+x]}, \overline{sm[t]}] \rangle$ ]
   $\langle OP[\overline{sp[t]}, \overline{sm[t]}] \rangle$ 
   $\langle OP[\overline{sp[t+2]}, \overline{sm[t]}] \rangle$ 
]

```

## ■ Derivation of the one-mode double time correlation result

```

In[28]:= expression1 = Assuming[δt > 0 && τ' > 0 ,
Collect[
  ⎧OP[OverBar[ad[t]] + i√ $\frac{2}{\tau'}$  OverBar[sp[t]],
    OverBar[ad[t + δt]] + i√ $\frac{2}{\tau'}$  OverBar[sp[t + δt]], OverBar[a[t + δt]] -
    i√ $\frac{2}{\tau'}$  OverBar[sm[t + δt]], OverBar[a[t]] - i√ $\frac{2}{\tau'}$  OverBar[sm[t]]⎫
  , {⟨a_[t1_]⟩, ⟨OP[a_[t1_], b_[t2_]]⟩, Conjugate[⟨OP[a_[t1_], b_[t2_]]⟩],
    ⟨OP[a_[t1_], b_[t2_], c_[t3_]]⟩}, Simplify]
]

Out[28]= 
$$\frac{(8 + \tau'^2 \omega^2)^2}{64 \tau'^2} - \frac{i e^{i(k t - \phi)} \omega^0 (8 + \tau'^2 \omega^2) \langle \overline{\text{sm}[t]} \rangle}{16 \tau'}$$


$$+ \frac{1}{16} i e^{i(k(t + \delta t) - \phi)} \tau' \omega^3 \langle \overline{\text{sm}[t + \delta t]} \rangle + \frac{i e^{-i k t + i \phi} \omega^0 (8 + \tau'^2 \omega^2) \langle \overline{\text{sp}[t]} \rangle}{16 \tau'}$$


$$+ \frac{1}{16} i e^{-i k(t + \delta t) + i \phi} \tau' \omega^3 \langle \overline{\text{sp}[t + \delta t]} \rangle + \left( \frac{1}{\tau'^2} + \frac{\omega^2}{8} \right) \langle \overline{\text{sz}[t]} \rangle + \frac{1}{8} \omega^2 \langle \overline{\text{sz}[t + \delta t]} \rangle -$$


$$\frac{1}{4} e^{i(k(2t + \delta t) - 2\phi)} \omega^2 \langle \text{OP}[\overline{\text{sm}[t + \delta t]}, \overline{\text{sm}[t]}] \rangle + \frac{1}{4} e^{i k \delta t} \omega^2 \langle \text{OP}[\overline{\text{sp}[t]}, \overline{\text{sm}[t + \delta t]}] \rangle -$$


$$\frac{1}{4} e^{-i(k(2t + \delta t) - 2\phi)} \omega^2 \langle \text{OP}[\overline{\text{sp}[t]}, \overline{\text{sp}[t + \delta t]}] \rangle + \frac{i e^{-i k t + i \phi} \omega^0 \langle \text{OP}[\overline{\text{sp}[t]}, \overline{\text{sz}[t + \delta t]}] \rangle}{2 \tau'}$$


$$+ \frac{1}{4} e^{-i k \delta t} \omega^2 \langle \text{OP}[\overline{\text{sp}[t + \delta t]}, \overline{\text{sm}[t]}] \rangle - \frac{i e^{i(k t - \phi)} \omega^0 \langle \text{OP}[\overline{\text{sz}[t + \delta t]}, \overline{\text{sm}[t]}] \rangle}{2 \tau'}$$


$$- \frac{1}{\tau'} i e^{i(k(t + \delta t) - \phi)} \omega^0 \langle \text{OP}[\overline{\text{sp}[t]}, \overline{\text{sm}[t + \delta t]}, \overline{\text{sm}[t]}] \rangle + \frac{1}{\tau'}$$


$$i e^{-i k(t + \delta t) + i \phi} \omega^0 \langle \text{OP}[\overline{\text{sp}[t]}, \overline{\text{sp}[t + \delta t]}, \overline{\text{sm}[t]}] \rangle + \frac{2 \langle \text{OP}[\overline{\text{sp}[t]}, \overline{\text{sz}[t + \delta t]}, \overline{\text{sm}[t]}] \rangle}{\tau'^2}$$


```

```

In[29]:= (* Manually take the laplace transform of the constant part *)

```

```

expression1[[1]] = expression1[[1]] *  $\frac{1}{s}$ ;

```

```

(* Various rules for different expectation values,
based on the solutions of the Bloch equations. *)

```

$$\text{ps} = \left( s + \frac{2}{\tau'} \right) \left( \left( s + \frac{1}{\tau'} \right)^2 + \delta \Omega^2 \right) + \omega^2 \left( s + \frac{1}{\tau'} \right);$$

$$\text{rule1} = \langle \overline{\text{sm}[\text{t}_-]} \rangle \rightarrow \frac{-\text{i} \omega 0 * \tau'}{2} \text{Exp}[-\text{i} k t + \text{i} \phi] \frac{1 - \text{i} * \delta \Omega * \tau'}{1 + (\delta \Omega * \tau')^2 + \frac{1}{2} (\omega 0 * \tau')^2} * \frac{1}{s};$$

$$\text{rule2} = \langle \overline{\text{sp}[\text{t}_-]} \rangle \rightarrow \frac{\text{i} \omega 0 * \tau'}{2} \text{Exp}[\text{i} k t - \text{i} \phi] \frac{1 + \text{i} * \delta \Omega * \tau'}{1 + (\delta \Omega * \tau')^2 + \frac{1}{2} (\omega 0 * \tau')^2} * \frac{1}{s};$$

$$\text{rule3} = \langle \overline{\text{sz}[\text{t}_-]} \rangle \rightarrow -\frac{1 + (\delta \Omega * \tau')^2}{1 + (\delta \Omega * \tau')^2 + \frac{1}{2} (\omega 0 * \tau')^2} * \frac{1}{s};$$

$$\text{rule4} = \langle \mathcal{OP}[\overline{\text{sp}[\text{t}]}, \overline{\text{sm}[\text{t} + \delta \text{t}]}] \rangle \rightarrow e^{-\text{i} k \delta t} \frac{\frac{1}{4} (\omega 0 * \tau')^2}{1 + (\delta \Omega * \tau')^2 + \frac{1}{2} (\omega 0 * \tau')^2} \frac{\text{ps} - \frac{1}{2} \omega 0^2 \left(s + \frac{2}{\tau'}\right)}{s * \text{ps}};$$

$$\text{rule5} = \langle \mathcal{OP}[\overline{\text{sp}[\text{t}]}, \overline{\text{sp}[\text{t} + \delta \text{t}]}] \rangle \rightarrow e^{\text{i} k \delta t} \frac{-\frac{1}{4} (\omega 0 * \tau')^2 e^{-2 \text{i} \phi} e^{2 \text{i} k * t}}{1 + (\delta \Omega * \tau')^2 + \frac{1}{2} (\omega 0 * \tau')^2}$$

$$\left( \frac{\text{ps} - \frac{1}{2} \omega 0^2 \left(s + \frac{2}{\tau'}\right)}{s * \text{ps}} \left( s + \frac{1}{\tau'} + \text{i} * \delta \Omega \right) - 1 \right) \frac{1}{\left(s + \frac{1}{\tau'} - \text{i} * \delta \Omega\right)};$$

$$\text{rule6} = \langle \mathcal{OP}[\overline{\text{sp}[\text{t}]}, \overline{\text{sz}[\text{t} + \delta \text{t}]}] \rangle \rightarrow \frac{-\frac{\text{i}}{2} \omega 0 * \tau',^2 * e^{-\text{i} \phi} e^{\text{i} k * t}}{1 + (\delta \Omega * \tau')^2 + \frac{1}{2} (\omega 0 * \tau')^2}$$

$$\left( \frac{\text{ps} - \frac{1}{2} \omega 0^2 \left(s + \frac{2}{\tau'}\right)}{s * \text{ps}} \left( s + \frac{1}{\tau'} + \text{i} * \delta \Omega \right) - 1 \right);$$

$$\text{rule7} = \langle \mathcal{OP}[\overline{\text{sp}[\text{t}]}, \overline{\text{sm}[\text{t} + \delta \text{t}]}, \overline{\text{sm}[\text{t}]}] \rangle \rightarrow e^{-\text{i} * k * (t + \delta t)} \frac{\frac{1}{4} (\omega 0 * \tau')^2}{1 + (\delta \Omega * \tau')^2 + \frac{1}{2} (\omega 0 * \tau')^2} \text{i} \frac{\omega 0}{2} e^{\text{i} * \phi} \frac{\left(-\frac{1}{s}\right) \left(s + \frac{2}{\tau'}\right) \left(s + \frac{1}{\tau'} - \text{i} * \delta \Omega\right)}{\text{ps}};$$

$$\text{rule8} = \langle \mathcal{OP}[\overline{\text{sp}[\text{t}]}, \overline{\text{sp}[\text{t} + \delta \text{t}]}, \overline{\text{sm}[\text{t}]}] \rangle \rightarrow e^{+\text{i} k (t + \delta t)} \frac{\frac{1}{4} (\omega 0 * \tau')^2}{1 + (\delta \Omega * \tau')^2 + \frac{1}{2} (\omega 0 * \tau')^2}$$

$$(-\text{i}) \frac{\omega 0}{2} e^{-\text{i} * \phi} \frac{\left(-\frac{1}{s}\right) \left(s + \frac{2}{\tau'}\right) \left(s + \frac{1}{\tau'} + \text{i} * \delta \Omega\right)}{\text{ps}};$$

$$\text{rule9} = \langle \mathcal{OP}[\overline{\text{sp}[\text{t}]}, \overline{\text{sz}[\text{t} + \delta \text{t}]}, \overline{\text{sm}[\text{t}]}] \rangle \rightarrow \frac{\frac{1}{4} (\omega 0 * \tau')^2}{1 + (\delta \Omega * \tau')^2 + \frac{1}{2} (\omega 0 * \tau')^2} \frac{\left(-\frac{1}{s}\right) \left(s + \frac{2}{\tau'}\right) \left(\left(s + \frac{1}{\tau'}\right)^2 + \delta \Omega^2\right)}{\text{ps}};$$

$$\text{rule10} = \langle \mathcal{OP}[\overline{\text{sm}[\text{t} + \delta \text{t}]}, \overline{\text{sm}[\text{t}]}] \rangle \rightarrow e^{-\text{i} k \delta t} \frac{-\frac{1}{4} (\omega 0 * \tau')^2 e^{2 \text{i} \phi} e^{-2 \text{i} k * t}}{1 + (\delta \Omega * \tau')^2 + \frac{1}{2} (\omega 0 * \tau')^2}$$

$$\left( \frac{ps - \frac{1}{2} \omega 0^2 \left( s + \frac{2}{\tau'} \right)}{s * ps} \left( s + \frac{1}{\tau'} - i * \delta \Omega \right) - 1 \right) \frac{1}{\left( s + \frac{1}{\tau'} + i * \delta \Omega \right)} ;$$

$$\text{rule11} = \langle \mathcal{OP}[\overline{\text{sp}[t + \delta t]}, \overline{\text{sm}[t]}] \rangle \rightarrow e^{i k \delta t} \frac{\frac{1}{4} (\omega 0 * \tau')^2}{1 + (\delta \Omega * \tau')^2 + \frac{1}{2} (\omega 0 * \tau')^2} \frac{ps - \frac{1}{2} \omega 0^2 \left( s + \frac{2}{\tau'} \right)}{s * ps} ;$$

$$\text{rule12} = \langle \mathcal{OP}[\overline{\text{sz}[t + \delta t]}, \overline{\text{sm}[t]}] \rangle \rightarrow \frac{+ \frac{1}{2} \omega 0 * \tau'^2 * e^{+i \phi} e^{-i k * t}}{1 + (\delta \Omega * \tau')^2 + \frac{1}{2} (\omega 0 * \tau')^2} \left( \frac{ps - \frac{1}{2} \omega 0^2 \left( s + \frac{2}{\tau'} \right)}{s * ps} \left( s + \frac{1}{\tau'} - i * \delta \Omega \right) - 1 \right) ;$$

```
rules = {rule1, rule2, rule3, rule4, rule5, rule6, rule7,
  rule8, rule9, rule10, rule11, rule12};
```

```
(* Apply the simplifications *)
```

```
Assuming[Element[δt, Reals] && Element[k, Reals] && Element[t, Reals],
```

```
dum = Simplify[expression1 //. rules]
```

```
]
```

$$\text{Out[44]} = \left( \tau'^2 \omega 0^4 \right. \\ \left( \left( 2 + 2 \delta \Omega^2 \tau'^2 + \tau'^2 \omega 0^2 \right)^2 + 4 s^2 \tau'^2 \left( 6 + 2 \delta \Omega^2 \tau'^2 + \tau'^2 \omega 0^2 \right) + s^3 \tau'^3 \left( 18 + 2 \delta \Omega^2 \tau'^2 + \tau'^2 \omega 0^2 \right) + \right. \\ \left. s \tau' \left( 10 + 2 \delta \Omega^4 \tau'^4 + 7 \tau'^2 \omega 0^2 + \tau'^4 \omega 0^4 + 3 \delta \Omega^2 \tau'^2 \left( 4 + \tau'^2 \omega 0^2 \right) \right) \right) \Big/ \left( 64 s \right. \\ \left. \left( 2 + 2 \delta \Omega^2 \tau'^2 + \tau'^2 \omega 0^2 \right) \left( 2 + 4 s^2 \tau'^2 + 2 \delta \Omega^2 \tau'^2 + s^3 \tau'^3 + \tau'^2 \omega 0^2 + s \tau' \left( 5 + \delta \Omega^2 \tau'^2 + \tau'^2 \omega 0^2 \right) \right) \right)$$

```
In[45]:= (* This is a massaged version of the longer output above. *)
```

$$\text{finalForm} = \frac{1}{s} + \frac{8}{1 + (\delta \Omega * \tau')^2 + \frac{1}{2} (\omega 0 * \tau')^2} \frac{s \left( s + \frac{1}{\tau'} \right)}{ps} ;$$

```
(* As you can see the two expressions are identical *)
```

$$\text{Simplify} \left[ \text{finalForm} - \text{ApartSquareFree} \left[ \frac{\text{dum}}{\frac{1}{\tau'^2} \frac{(\omega 0 * \tau')^4}{64}}, s \right] \right]$$

```
Out[46]= 0
```

## ■ Derivation of the two-mode double time correlation result

### ■ Transmission

In[47]:= `expression2 = Assuming[ $\delta t > 0 \ \&\& \ \tau' > 0$ ,`

`Collect[`

$$\begin{aligned} & \frac{1}{4} \left\langle \mathcal{OP} \left[ \overline{\text{ad}[t]} + i \sqrt{\frac{2}{\tau'}} \overline{\text{sp}[t]} + \frac{\omega_0}{2} \sqrt{\frac{\tau'}{2}} e^{-i\phi} e^{ik t}, \right. \right. \\ & \quad \overline{\text{ad}[t + \delta t]} + i \sqrt{\frac{2}{\tau'}} \overline{\text{sp}[t + \delta t]} + \frac{\omega_0}{2} \sqrt{\frac{\tau'}{2}} e^{-i\phi} e^{ik(t + \delta t)}, \\ & \quad \overline{\text{a}[t + \delta t]} - i \sqrt{\frac{2}{\tau'}} \overline{\text{sm}[t + \delta t]} + \frac{\omega_0}{2} \sqrt{\frac{\tau'}{2}} e^{+i\phi} e^{-ik(t + \delta t)}, \\ & \quad \left. \overline{\text{a}[t]} - i \sqrt{\frac{2}{\tau'}} \overline{\text{sm}[t]} + \frac{\omega_0}{2} \sqrt{\frac{\tau'}{2}} e^{+i\phi} e^{-ik t} \right] \Bigg\rangle \\ & , \{ \langle \overline{\text{a}[t_1]} \rangle, \langle \mathcal{OP}[\overline{\text{a}[t_1]}, \overline{\text{b}[t_2]}] \rangle, \text{Conjugate}[\langle \mathcal{OP}[\overline{\text{a}[t_1]}, \overline{\text{b}[t_2]}] \rangle], \\ & \quad \langle \mathcal{OP}[\overline{\text{a}[t_1]}, \overline{\text{b}[t_2]}, \overline{\text{c}[t_3]}] \rangle \}, \text{Simplify} \Big] \end{aligned}$$

`]`

$$\begin{aligned} \text{Out[47]} = & \frac{(2 + \tau'^2 \omega_0^2)^2}{16 \tau'^2} - \frac{i e^{i(k t - \phi)} \omega_0 (2 + \tau'^2 \omega_0^2) \langle \overline{\text{sm}[t]} \rangle}{8 \tau'} - \\ & \frac{1}{8} i e^{i(k(t + \delta t) - \phi)} \tau' \omega_0^3 \langle \overline{\text{sm}[t + \delta t]} \rangle + \frac{i e^{-i k t + i \phi} \omega_0 (2 + \tau'^2 \omega_0^2) \langle \overline{\text{sp}[t]} \rangle}{8 \tau'} + \\ & \frac{1}{8} i e^{-i k(t + \delta t) + i \phi} \tau' \omega_0^3 \langle \overline{\text{sp}[t + \delta t]} \rangle + \frac{1}{4} \left( \frac{1}{\tau'^2} + \frac{\omega_0^2}{2} \right) \langle \overline{\text{sz}[t]} \rangle + \frac{1}{8} \omega_0^2 \langle \overline{\text{sz}[t + \delta t]} \rangle - \\ & \frac{1}{4} e^{i(k(2t + \delta t) - 2\phi)} \omega_0^2 \langle \mathcal{OP}[\overline{\text{sm}[t + \delta t]}, \overline{\text{sm}[t]}] \rangle + \frac{1}{4} e^{i k \delta t} \omega_0^2 \langle \mathcal{OP}[\overline{\text{sp}[t]}, \overline{\text{sm}[t + \delta t]}] \rangle - \\ & \frac{1}{4} e^{-i(k(2t + \delta t) - 2\phi)} \omega_0^2 \langle \mathcal{OP}[\overline{\text{sp}[t]}, \overline{\text{sp}[t + \delta t]}] \rangle + \frac{i e^{-i k t + i \phi} \omega_0 \langle \mathcal{OP}[\overline{\text{sp}[t]}, \overline{\text{sz}[t + \delta t]}] \rangle}{4 \tau'} + \\ & \frac{1}{4} e^{-i k \delta t} \omega_0^2 \langle \mathcal{OP}[\overline{\text{sp}[t + \delta t]}, \overline{\text{sm}[t]}] \rangle - \frac{i e^{i(k t - \phi)} \omega_0 \langle \mathcal{OP}[\overline{\text{sz}[t + \delta t]}, \overline{\text{sm}[t]}] \rangle}{4 \tau'} - \\ & \frac{1}{2 \tau'} i e^{i(k(t + \delta t) - \phi)} \omega_0 \langle \mathcal{OP}[\overline{\text{sp}[t]}, \overline{\text{sm}[t + \delta t]}, \overline{\text{sm}[t]}] \rangle + \frac{1}{2 \tau'} \\ & i e^{-i k(t + \delta t) + i \phi} \omega_0 \langle \mathcal{OP}[\overline{\text{sp}[t]}, \overline{\text{sp}[t + \delta t]}, \overline{\text{sm}[t]}] \rangle + \frac{\langle \mathcal{OP}[\overline{\text{sp}[t]}, \overline{\text{sz}[t + \delta t]}, \overline{\text{sm}[t]}] \rangle}{2 \tau'^2} \end{aligned}$$

In[48]:= (\* Manually take the laplace transform of the constant part \*)

expression2[[1]] = expression2[[1]] \*  $\frac{1}{s}$ ;

expression2

$$\begin{aligned} \text{Out[49]} = & \frac{(2 + \tau'^2 \omega 0^2)^2}{16 s \tau'^2} - \frac{i e^{i(k t - \phi)} \omega 0 (2 + \tau'^2 \omega 0^2) \langle \overline{\text{sm}[t]} \rangle}{8 \tau'} - \\ & \frac{1}{8} i e^{i(k(t + \delta t) - \phi)} \tau' \omega 0^3 \langle \overline{\text{sm}[t + \delta t]} \rangle + \frac{i e^{-i k t + i \phi} \omega 0 (2 + \tau'^2 \omega 0^2) \langle \overline{\text{sp}[t]} \rangle}{8 \tau'} + \\ & \frac{1}{8} i e^{-i k(t + \delta t) + i \phi} \tau' \omega 0^3 \langle \overline{\text{sp}[t + \delta t]} \rangle + \frac{1}{4} \left( \frac{1}{\tau'^2} + \frac{\omega 0^2}{2} \right) \langle \overline{\text{sz}[t]} \rangle + \frac{1}{8} \omega 0^2 \langle \overline{\text{sz}[t + \delta t]} \rangle - \\ & \frac{1}{4} e^{i(k(2t + \delta t) - 2\phi)} \omega 0^2 \langle \mathcal{OP}[\overline{\text{sm}[t + \delta t]}, \overline{\text{sm}[t]}] \rangle + \frac{1}{4} e^{i k \delta t} \omega 0^2 \langle \mathcal{OP}[\overline{\text{sp}[t]}, \overline{\text{sm}[t + \delta t]}] \rangle - \\ & \frac{1}{4} e^{-i(k(2t + \delta t) - 2\phi)} \omega 0^2 \langle \mathcal{OP}[\overline{\text{sp}[t]}, \overline{\text{sp}[t + \delta t]}] \rangle + \frac{i e^{-i k t + i \phi} \omega 0 \langle \mathcal{OP}[\overline{\text{sp}[t]}, \overline{\text{sz}[t + \delta t]}] \rangle}{4 \tau'} + \\ & \frac{1}{4} e^{-i k \delta t} \omega 0^2 \langle \mathcal{OP}[\overline{\text{sp}[t + \delta t]}, \overline{\text{sm}[t]}] \rangle - \frac{i e^{i(k t - \phi)} \omega 0 \langle \mathcal{OP}[\overline{\text{sz}[t + \delta t]}, \overline{\text{sm}[t]}] \rangle}{4 \tau'} - \\ & \frac{1}{2 \tau'} i e^{i(k(t + \delta t) - \phi)} \omega 0 \langle \mathcal{OP}[\overline{\text{sp}[t]}, \overline{\text{sm}[t + \delta t]}, \overline{\text{sm}[t]}] \rangle + \frac{1}{2 \tau'} \\ & i e^{-i k(t + \delta t) + i \phi} \omega 0 \langle \mathcal{OP}[\overline{\text{sp}[t]}, \overline{\text{sp}[t + \delta t]}, \overline{\text{sm}[t]}] \rangle + \frac{\langle \mathcal{OP}[\overline{\text{sp}[t]}, \overline{\text{sz}[t + \delta t]}, \overline{\text{sm}[t]}] \rangle}{2 \tau'^2} \end{aligned}$$

In[50]:= expression2norm =

Assuming[t > 0 && δt > 0 && τ' > 0 && ω0 > 0 && k > 0 && Element[φ, Reals],

Collect[

$$\frac{1}{2} \left\langle \mathcal{OP}[\overline{\text{ad}[t]}] + i \sqrt{\frac{2}{\tau'}} \overline{\text{ad}[t]} + \frac{\omega 0}{2} \sqrt{\frac{\tau'}{2}} e^{-i \phi} e^{i k t}, \right.$$

$$\left. \overline{\text{a}[t]} - i \sqrt{\frac{2}{\tau'}} \overline{\text{sm}[t]} + \frac{\omega 0}{2} \sqrt{\frac{\tau'}{2}} e^{+i \phi} e^{-i k t} \right\rangle$$

$$, \{ \langle \overline{\text{a}[t1]} \rangle, \langle \mathcal{OP}[\overline{\text{a}[t1]}, \overline{\text{b}[t2]}] \rangle, \text{Conjugate}[\langle \mathcal{OP}[\overline{\text{a}[t1]}, \overline{\text{b}[t2]}] \rangle], \\ \langle \mathcal{OP}[\overline{\text{a}[t1]}, \overline{\text{b}[t2]}, \overline{\text{c}[t3]}] \rangle \}, \text{Simplify}]$$

$$\text{Out[50]} = \frac{2 + \tau'^2 \omega 0^2}{4 \tau'} - \frac{1}{2} i e^{i(k t - \phi)} \omega 0 \langle \overline{\text{sm}[t]} \rangle + \frac{1}{2} i e^{-i k t + i \phi} \omega 0 \langle \overline{\text{sp}[t]} \rangle + \frac{\langle \overline{\text{sz}[t]} \rangle}{2 \tau'}$$



```
In[51]:= expression2norm[[1]] = expression2norm[[1]] *  $\frac{1}{s}$ ;
```

```
expression2norm
```

```
Out[52]= 
$$\frac{2 + \tau'^2 \omega 0^2}{4 s \tau'} - \frac{1}{2} i e^{i(k t - \phi)} \omega 0 \langle \overline{\text{sm}[\tau]} \rangle + \frac{1}{2} i e^{-i k t + i \phi} \omega 0 \langle \overline{\text{sp}[\tau]} \rangle + \frac{\langle \overline{\text{sz}[\tau]} \rangle}{2 \tau'}$$

```

```
In[53]:= Assuming[Element[δt, Reals] && Element[k, Reals] && Element[t, Reals],
  expression2norm = Simplify[expression2norm /. rules];
]
```

```
expression2norm = expression2norm * s
```

```
Out[54]= 
$$\frac{\tau'^3 \omega 0^2 (2 \delta \Omega^2 + \omega 0^2)}{4 (2 + 2 \delta \Omega^2 \tau'^2 + \tau'^2 \omega 0^2)}$$

```

```
In[55]:= Assuming[Element[δt, Reals] && Element[k, Reals] && Element[t, Reals],
  dum = Simplify[expression2 /. rules];
]
```

```
In[56]:= ApartSquareFree[ $\frac{\text{dum}}{\text{expression2norm}^2}$ , s]
```

```
Out[56]= 
$$\frac{1}{s} + \frac{(4 (1 + 2 s \tau' + s^2 \tau'^2 + 5 \delta \Omega^2 \tau'^2 + 6 s \delta \Omega^2 \tau'^3 + 2 s^2 \delta \Omega^2 \tau'^4 + 2 \tau'^2 \omega 0^2 + 3 s \tau'^3 \omega 0^2 + s^2 \tau'^4 \omega 0^2))}{(\tau'^3 (2 \delta \Omega^2 + \omega 0^2)^2 (2 + 5 s \tau' + 4 s^2 \tau'^2 + 2 \delta \Omega^2 \tau'^2 + s^3 \tau'^3 + s \delta \Omega^2 \tau'^3 + \tau'^2 \omega 0^2 + s \tau'^3 \omega 0^2))}$$

```

```
In[57]:= A =  $\delta \Omega^2 \tau'^2 + \frac{1}{2} \omega 0^2 \tau'^2$ ;
```

```
finalForm =  $\frac{1}{s} + \frac{1}{A^2} \frac{1}{ps} \left( \left( s + \frac{1}{\tau'} \right) \left( (1 + 2 A) s + \frac{1 + 4 A}{\tau'} \right) + \delta \Omega^2 \right)$ ;
```

```
Simplify[finalForm - ApartSquareFree[ $\frac{\text{dum}}{\text{expression2norm}^2}$ , s]]
```

```
Out[59]= 0
```

## ■ Reflection

```

In[70]:= expression3 = Assuming[δt > 0 && τ' > 0 ,
Collect[


$$\frac{1}{4} \left\langle \mathcal{OP} \left[ \overline{\text{ad}[t]} + i \sqrt{\frac{2}{\tau'}} \overline{\text{sp}[t]} - \frac{\omega 0}{2} \sqrt{\frac{\tau'}{2}} e^{-i \phi} e^{i k t}, \right. \right.$$



$$\overline{\text{ad}[t + \delta t]} + i \sqrt{\frac{2}{\tau'}} \overline{\text{sp}[t + \delta t]} - \frac{\omega 0}{2} \sqrt{\frac{\tau'}{2}} e^{-i \phi} e^{i k (t + \delta t)},$$



$$\overline{\text{a}[t + \delta t]} - i \sqrt{\frac{2}{\tau'}} \overline{\text{sm}[t + \delta t]} - \frac{\omega 0}{2} \sqrt{\frac{\tau'}{2}} e^{+i \phi} e^{-i k (t + \delta t)},$$



$$\left. \overline{\text{a}[t]} - i \sqrt{\frac{2}{\tau'}} \overline{\text{sm}[t]} - \frac{\omega 0}{2} \sqrt{\frac{\tau'}{2}} e^{+i \phi} e^{-i k t} \right\rangle$$


, {⟨ $\overline{\text{a}[t1]}$ ⟩, ⟨ $\mathcal{OP}[\overline{\text{a}[t1]}, \overline{\text{b}[t2]}$ ⟩, Conjugate[⟨ $\mathcal{OP}[\overline{\text{a}[t1]}, \overline{\text{b}[t2]}$ ⟩]⟩,
⟨ $\mathcal{OP}[\overline{\text{a}[t1]}, \overline{\text{b}[t2]}, \overline{\text{c}[t3]}$ ⟩]⟩}, Simplify]

]

Out[70]=  $\frac{1}{4 \tau'^2} + \frac{\langle \overline{\text{sz}[t]} \rangle}{4 \tau'^2} + \frac{\langle \mathcal{OP}[\overline{\text{sp}[t]}, \overline{\text{sz}[t + \delta t]}, \overline{\text{sm}[t]}] \rangle}{2 \tau'^2}$ 

In[71]:= (* Manually take the laplace transform of the constant *)

expression3[[1]] = expression3[[1]] *  $\frac{1}{s}$ ;

expression3

Out[72]=  $\frac{1}{4 s \tau'^2} + \frac{\langle \overline{\text{sz}[t]} \rangle}{4 \tau'^2} + \frac{\langle \mathcal{OP}[\overline{\text{sp}[t]}, \overline{\text{sz}[t + \delta t]}, \overline{\text{sm}[t]}] \rangle}{2 \tau'^2}$ 

```

```
In[73]:= expression3norm =
  Assuming[t > 0 && δt > 0 && τ' > 0 && ω0 > 0 && k > 0 && Element[φ, Reals],
  Collect[
    
$$\frac{1}{2} \left\langle \mathcal{OP} \left[ \overline{\text{ad}[t]} + i \sqrt{\frac{2}{\tau'}} \overline{\text{sp}[t]} - \frac{\omega 0}{2} \sqrt{\frac{\tau'}{2}} e^{-i\phi} e^{ik t}, \right. \right.$$


$$\left. \overline{\text{a}[t]} - i \sqrt{\frac{2}{\tau'}} \overline{\text{sm}[t]} - \frac{\omega 0}{2} \sqrt{\frac{\tau'}{2}} e^{+i\phi} e^{-ik t} \right\rangle$$


$$, \{ \langle \overline{\text{a}[t1_]}, \overline{\text{a}[t1_], \text{b}[t2_]} \rangle, \text{Conjugate}[\langle \mathcal{OP}[\overline{\text{a}[t1_], \text{b}[t2_]}] \rangle],$$


$$\langle \mathcal{OP}[\overline{\text{a}[t1_], \text{b}[t2_], \text{c}[t3_]}] \rangle \}, \text{Simplify}$$

  ]
```

$$\text{Out[73]} = \frac{1}{2 \tau'} + \frac{\langle \overline{\text{sz}[t]} \rangle}{2 \tau'}$$

```
In[74]:= expression3norm[[1]] = expression3norm[[1]] *  $\frac{1}{s}$ ;
expression3norm
```

$$\text{Out[75]} = \frac{1}{2 s \tau'} + \frac{\langle \overline{\text{sz}[t]} \rangle}{2 \tau'}$$

```
In[76]:= Assuming[Element[δt, Reals] && Element[k, Reals] && Element[t, Reals],
  expression3norm = Simplify[expression3norm /. rules];
]
expression3norm = expression3norm * s
```

$$\text{Out[77]} = \frac{s \tau' \omega 0^2}{4 s + 4 s \delta \Omega^2 \tau'^2 + 2 s \tau'^2 \omega 0^2}$$

```
In[78]:= Assuming[Element[δt, Reals] && Element[k, Reals] && Element[t, Reals],
  dum = Simplify[expression3 /. rules];
]
```

```
In[79]:= ApartSquareFree[ $\frac{\text{dum}}{\text{expression3norm}^2}$ , s]
```

$$\text{Out[79]} = \frac{1}{s} + \left( -3 \tau' - 4 s \tau'^2 - s^2 \tau'^3 + \delta \Omega^2 \tau'^3 \right) /$$

$$\left( 2 + 5 s \tau' + 4 s^2 \tau'^2 + 2 \delta \Omega^2 \tau'^2 + s^3 \tau'^3 + s \delta \Omega^2 \tau'^3 + \tau'^2 \omega 0^2 + s \tau'^3 \omega 0^2 \right)$$

```
In[80]:= finalForm =  $\frac{2}{\tau'^2} \left( 1 + (\delta\Omega * \tau')^2 + \frac{1}{2} (\omega_0 * \tau')^2 \right) \frac{s + \frac{1}{\tau'}}{s * ps};$ 
Simplify[finalForm - ApartSquareFree[ $\frac{\text{dum}}{\text{expression3norm}^2}, s$ ]]
```

Out[81]= 0

## Code for Fig1

### ■ Coherent part

```
In[82]:= Tcoh[D_, R_] :=
  1 / (1 + D^2 + 1 / 2 R^2) (D^2 + 1 / 2 R^2 (D^2 + 1 / 2 R^2) / (1 + D^2 + 1 / 2 R^2));
Rcoh[D_, R_] := (1 + D^2) / (1 + D^2 + 1 / 2 R^2)^2;
P[s_, D_, R_] := s^3 + s (5 + R^2 + D^2) + 2 + R^2 + 2 D^2 + 4 s^2;
Tinc[w_, D_, R_] :=  $\frac{1}{\pi} \frac{1}{(1 + D^2 + 1 / 2 R^2)} \frac{R^2 (w^2 + 4 + 1 / 2 R^2)}{P[-I w, D, R] P[I w, D, R]}$ ;
fig1p1 = Plot[{Tcoh[w, 0.1], Tcoh[w, 2], Tcoh[w, 5]},
  {w, -10, 10}, PlotRange -> All, Axes -> False, Frame -> True];
fig1p2 = Plot[{Rcoh[w, 0.1], Rcoh[w, 2], 5 Rcoh[w, 5]}, {w, -10, 10}, PlotRange -> All,
  PlotStyle -> Dashed, Axes -> False, Frame -> True, Epilog -> Text["x5", {8, 0.1}]];
Show[fig1p2, fig1p1]
```

Out[88]=

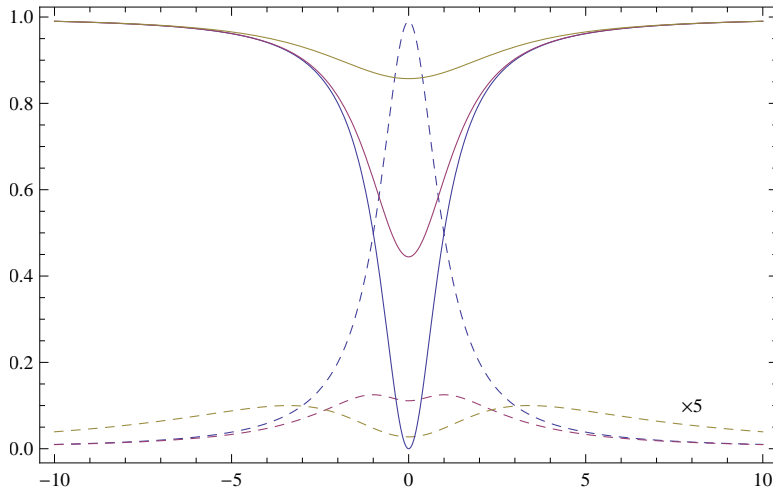

## ■ Incoherent part

```
In[89]:= DensityPlot[Log[10, Tinc[w, 0, 10^R]], {R, 0, 2}, {w, -50, 50}, PlotPoints → 100,
  ColorFunction → "FuchsiaTones", ImageSize → 72 * 3.4, BaseStyle → {FontSize → 8},
  FrameTicks → {{Automatic, None}, {{0, 1}, {Log[10, 2], 2}, {Log[10, 5], 5}, {1, 10},
    {Log[10, 20], 20}, {Log[10, 50], 50}, {2, 100}}}, None}}, Frame → False]
Export["insetRaw.png", %, ImageResolution → 300]
```

Out[89]=

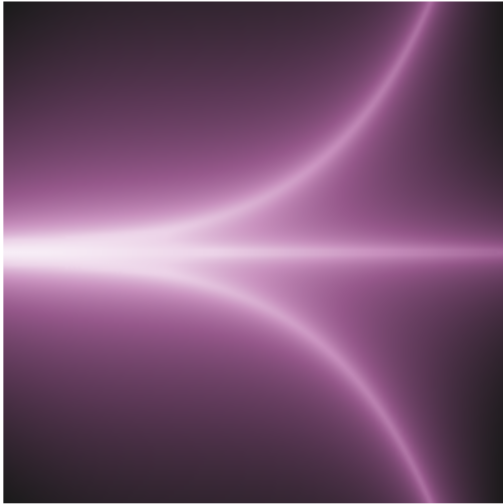

Out[90]= insetRaw.png

## ■ Data output for TikZ

```
In[91]:= lims = 10;
Export["Fig1Curve1.dat",
  Table[{coord, Tcoh[coord, 0.1]} // N, {coord, -lims, lims, lims / 100}], "Table"]
Export["Fig1Curve2.dat", Table[{coord, Tcoh[coord, 2]} // N,
  {coord, -lims, lims, lims / 100}], "Table"]
Export["Fig1Curve3.dat", Table[{coord, Tcoh[coord, 5]} // N,
  {coord, -lims, lims, lims / 100}], "Table"]
Export["Fig1Curve4.dat", Table[{coord, Rcoh[coord, 0.1]} // N,
  {coord, -lims, lims, lims / 100}], "Table"]
Export["Fig1Curve5.dat", Table[{coord, Rcoh[coord, 2]} // N,
  {coord, -lims, lims, lims / 100}], "Table"]
Export["Fig1Curve6.dat", Table[{coord, 5 Rcoh[coord, 5]} // N,
  {coord, -lims, lims, lims / 100}], "Table"]

Out[92]= Fig1Curve1.dat
Out[93]= Fig1Curve2.dat
Out[94]= Fig1Curve3.dat
Out[95]= Fig1Curve4.dat
Out[96]= Fig1Curve5.dat
Out[97]= Fig1Curve6.dat
```

---

## Code for Fig2

```
In[98]:= delOmega = 2;
rabiFreqa = 0.2;
rabiFreqb = 4;
phi = 0;

(* one-way *)
g2oneway[ΔΩ_, ωr_, φ_, t_] := Module[{τ, ps},
  τ = 1;
  ps =  $\left(s + \frac{2}{\tau}\right) \left(\left(s + \frac{1}{\tau}\right)^2 + \Delta\Omega^2\right) + \omega r^2 \left(s + \frac{1}{\tau}\right);$ 
  InverseLaplaceTransform $\left[\frac{1}{s} + \frac{8}{1 + \Delta\Omega^2 \tau^2 + \frac{1}{2} \omega r^2 \tau^2} \frac{s \left(s + \frac{1}{\tau}\right)}{ps}, s, t\right]$ , s, t]
]
expression1aTest = g2oneway[delOmega, rabiFreqa, phi, δt];
expression1bTest = g2oneway[delOmega, rabiFreqb, phi, δt];

(* Transmitted *)
```

```

g2twayT[ΔΩ_, ωr_, ϕ_, t_] := Module[{τ, ps, A},
  τ = 1;
  A = ΔΩ² τ² + 1/2 ωr² τ²;
  ps = (s + 2/τ) ( (s + 1/τ)² + ΔΩ² ) + ωr² (s + 1/τ);
  InverseLaplaceTransform[1/s + 1/A² 1/ps ( (s + 1/τ) ( (1 + 2 A) s + 1 + 4 A/τ ) + ΔΩ² ), s, t]
]
expression2aTest = g2twayT[delOmega, rabiFreqa, phi, δt];
expression2bTest = g2twayT[delOmega, rabiFreqb, phi, δt];

(* Reflected *)
g2twayR[ΔΩ_, ωr_, ϕ_, t_] := Module[{τ, ps},
  τ = 1;
  ps = (s + 2/τ) ( (s + 1/τ)² + ΔΩ² ) + ωr² (s + 1/τ);
  InverseLaplaceTransform[2 * (1 + ΔΩ² τ² + 1/2 ωr² τ²) 1/τ² (s + 1/τ)/(s * ps), s, t]
]
expression3aTest = g2twayR[delOmega, rabiFreqa, phi, δt];
expression3bTest = g2twayR[delOmega, rabiFreqb, phi, δt];

(* Two-photon comparison *)
ψoneway[δΩ_, x_] := (sqrt(2)/(2 π) ( 4 e^(-Abs[x]) e^(-i δΩ Abs[x]) / (-δΩ + i)² + (-δΩ - i)² )) / (sqrt(2)/(2 π) (-δΩ - i)²);
ψtwayT[δΩ_, x_] := (sqrt(2)/(2 π) ( e^(-Abs[x]) e^(-i δΩ Abs[x]) / (-δΩ + i)² + 1/4 (-δΩ - i + 1)² )) / (sqrt(2)/(2 π) 1/4 (-δΩ - i + 1)²); (* Transmitted *)
ψtwayR[δΩ_, x_] := (sqrt(2)/(2 π) ( e^(-Abs[x]) e^(-i δΩ Abs[x]) / (-δΩ + i)² + 1/4 (-δΩ - i - 1)² )) / (sqrt(2)/(2 π) 1/4 (-δΩ - i - 1)²); (* Reflected *)

fig2p1 = Plot[{expression1aTest /. δt → Abs[t] // Chop,
  expression1bTest /. δt → Abs[t] // Chop, Abs[ψoneway[delOmega, t]]²},
{t, -10, 10}, PlotRange → All, Axes → False, Frame → True,
PlotStyle → {{Red}, {Black}, {Dashed, Blue}}, ImageSize → 72 * 4,
BaseStyle → {FontSize → 8}, FrameLabel → {δt, , "one-mode"}]
fig2p2 = Plot[{expression2aTest /. δt → Abs[t] // Chop,

```

```

expression2bTest /.  $\delta t \rightarrow \text{Abs}[t] \text{ // Chop, Abs}[\psi_{\text{twowayT}}[\text{delOmega}, t]]^2 \},$ 
{t, -10, 10}, PlotRange  $\rightarrow$  All, Axes  $\rightarrow$  False, Frame  $\rightarrow$  True,
PlotStyle  $\rightarrow$  {{Red}, {Black}, {Dashed, Blue}}, ImageSize  $\rightarrow$  72 * 4,
BaseStyle  $\rightarrow$  {FontSize  $\rightarrow$  8}, FrameLabel  $\rightarrow$  { $\delta t$ , , "two-mode transmitted"}]
fig2p3 = Plot[{expression3aTest /.  $\delta t \rightarrow \text{Abs}[t] \text{ // Chop,}$ 
expression3bTest /.  $\delta t \rightarrow \text{Abs}[t] \text{ // Chop, Abs}[\psi_{\text{twowayR}}[\text{delOmega}, t]]^2 \},$ 
{t, -10, 10}, PlotRange  $\rightarrow$  All, Axes  $\rightarrow$  False, Frame  $\rightarrow$  True,
PlotStyle  $\rightarrow$  {{Red}, {Black}, {Dashed, Blue}}, ImageSize  $\rightarrow$  72 * 4,
BaseStyle  $\rightarrow$  {FontSize  $\rightarrow$  8}, FrameLabel  $\rightarrow$  { $\delta t$ , , "two-mode reflected"}]

```

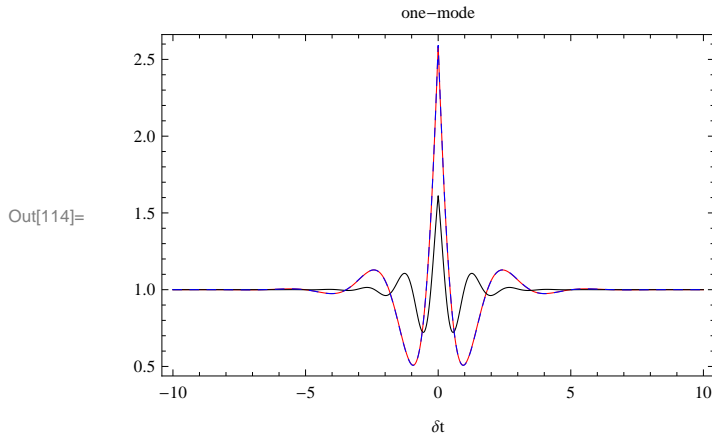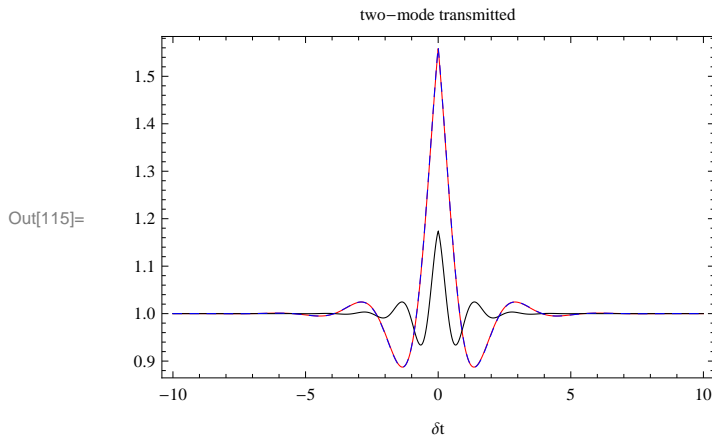



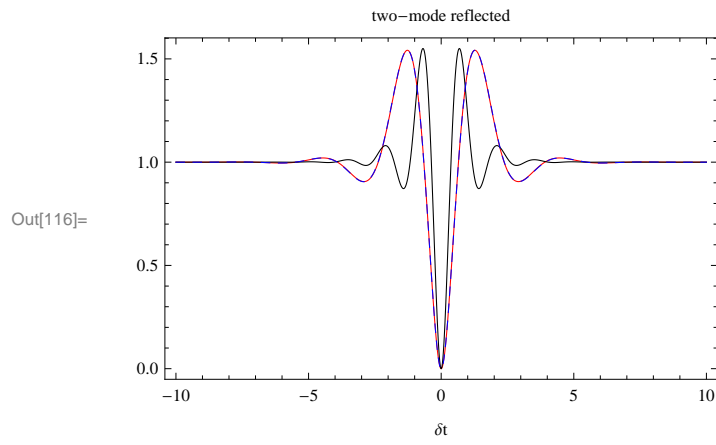

```

In[117]:= (* Data output for TikZ *)
lims = 6;
Export["Fig2aCurve1.dat", Table[{coord, expression1aTest /.  $\delta t \rightarrow \text{Abs}[\text{coord}]$ } // N,
  {coord, -lims, lims, lims / 100}] // Chop, "Table"]
Export["Fig2aCurve2.dat", Table[{coord, expression1bTest /.  $\delta t \rightarrow \text{Abs}[\text{coord}]$ } // N,
  {coord, -lims, lims, lims / 100}] // Chop, "Table"]
Export["Fig2aCurve3.dat", Table[{coord, Abs[ $\psi_{\text{oneway}}[2, t]^2$ ] /.  $t \rightarrow \text{coord}$ } // N,
  {coord, -lims, lims, lims / 100}], "Table"]

Export["Fig2bCurve1.dat", Table[{coord, expression2aTest /.  $\delta t \rightarrow \text{Abs}[\text{coord}]$ } // N,
  {coord, -lims, lims, lims / 100}] // Chop, "Table"]
Export["Fig2bCurve2.dat", Table[{coord, expression2bTest /.  $\delta t \rightarrow \text{Abs}[\text{coord}]$ } // N,
  {coord, -lims, lims, lims / 100}] // Chop, "Table"]
Export["Fig2bCurve3.dat", Table[{coord, Abs[ $\psi_{\text{two-wayT}}[2, t]^2$ ] /.  $t \rightarrow \text{coord}$ } // N,
  {coord, -lims, lims, lims / 100}], "Table"]

Export["Fig2cCurve1.dat", Table[{coord, expression3aTest /.  $\delta t \rightarrow \text{Abs}[\text{coord}]$ } // N,
  {coord, -lims, lims, lims / 100}] // Chop, "Table"]
Export["Fig2cCurve2.dat", Table[{coord, expression3bTest /.  $\delta t \rightarrow \text{Abs}[\text{coord}]$ } // N,
  {coord, -lims, lims, lims / 100}] // Chop, "Table"]
Export["Fig2cCurve3.dat", Table[{coord, Abs[ $\psi_{\text{two-wayR}}[2, t]^2$ ] /.  $t \rightarrow \text{coord}$ } // N,
  {coord, -lims, lims, lims / 100}], "Table"]

Out[118]= Fig2aCurve1.dat
Out[119]= Fig2aCurve2.dat
Out[120]= Fig2aCurve3.dat
Out[121]= Fig2bCurve1.dat
Out[122]= Fig2bCurve2.dat
Out[123]= Fig2bCurve3.dat
Out[124]= Fig2cCurve1.dat
Out[125]= Fig2cCurve2.dat
Out[126]= Fig2cCurve3.dat

```
